# Supplementary material for: SemEval-2024 Shared Task 6: SHROOM, a Shared-task on Hallucinations and Related Observable Overgeneration Mistakes
Source: arXiv:2403.07726 source file (2024-03-29)
Supplement: Supplementary file 1 [file annot_guidelines.pdf]

# Annotation guidelines for SHROOM

---

Thank you for agreeing to participate in the SHROOM survey! The present document will provide you some general guidelines as to what is expected of you.

## What are we looking for?

Our goal is to assess the **truthfulness** of sentences and documents written with artificial intelligence. In particular, we are interested in cases when the **AI outputs** are not supported by the facts. Such unsupported outputs are colloquially referred to as '**hallucinations**'.

You will be presented with a series of items. Each item contains an **AI output**, as well as one or more **References**, i.e., examples of what the model should have produced in an ideal scenario. Outputs and references can correspond to different types of sentences and paragraphs: news headlines, dictionary definitions, movie subtitles... We ask that **you mark for every item**, whether the output contains or describes facts that are **not supported by the provided reference**. Such items are instances of hallucinations.

In other words: **hallucinations are cases where the AI output is more specific than it should be, given the available reference.**

## Some Examples and counterexamples Hallucinations

---

### Hallucinations

Below are some examples of items our research team unanimously considered as hallucinations:

#### Example 1

Reference: The worship of trees.

AI output: (uncountable) The study of trees.

#### Example 2

Reference: Why is everyone laughing?

AI output: Why is everyone okay?

#### Example 3

Reference: You're a scam artist.

AI output: You're not a good scam artist.

### Not Hallucinations

And next, here are a few items that we unanimously did not consider as hallucinations:

#### Example 1

Reference: Capable of being deployed by parachute.

AI output: Capable of being parachuted.

## Example 2

Reference: When did you see him?

AI output: When was the last time you saw him?

## One last thing: Hallucinations vs. undergeneration

---

In some instances, the AI output can contain **less** information than the reference. We refer to such items as cases of **"undergeneration"**. These are not necessarily cases of hallucinations: as long as what is stated in the AI output is supported by the reference, such items should not be marked as hallucinations.

Here is one straightforward example:

Reference: I can't do it alone. You have to help me.

AI output: I can't do it alone.

Given that all the information present in the AI output is also found in the reference, **this should not be marked as a hallucination.**

**That's it!**
